# Supplementary material for: Inferring the joint demographic history of multiple populations from multidimensional SNP frequency data
Source: arXiv:0909.0925 source file (2009-09-04)
Supplement: Supplementary file 1 [file SupportingInformation.pdf]

# Inferring Human Divergence and Migration from Joint DNA Polymorphism Data

Supporting Information

Ryan N. Gutenkunst, Ryan D. Hernandez, Scott H. Williamson, & Carlos D. Bustamante

## Contents

**1 Properties of the AFS** **2**
1.1 Distinguishing reduced divergence and increased migration . . . . . . . . . . . 2

**2 Numerical methods** **3**
2.1 Finite-difference scheme . . . . . . . . . . . . . . . . . . . . . . . . . . . . 3
2.2 Population splits . . . . . . . . . . . . . . . . . . . . . . . . . . . . . . . . 4
2.3 Non-uniform grid . . . . . . . . . . . . . . . . . . . . . . . . . . . . . . . 5
2.4 Extrapolation . . . . . . . . . . . . . . . . . . . . . . . . . . . . . . . . . 5
2.5 Small-$M$ comparison with *ms* . . . . . . . . . . . . . . . . . . . . . . . . 6

**3 Data processing** **7**
3.1 Projection . . . . . . . . . . . . . . . . . . . . . . . . . . . . . . . . . . . 7
3.2 LD calculation . . . . . . . . . . . . . . . . . . . . . . . . . . . . . . . . . 8
3.3 Estimating $\mu$ . . . . . . . . . . . . . . . . . . . . . . . . . . . . . . . . . 8

**4 Coalescent simulations** **8**
4.1 Reduction of effective independent SNPs by linkage . . . . . . . . . . . . . 9

**5 Out of Africa model** **9**
5.1 Marginal analyses . . . . . . . . . . . . . . . . . . . . . . . . . . . . . . . 9
5.2 Maximum likelihood parameters . . . . . . . . . . . . . . . . . . . . . . . . 10
5.3 Projection and residuals . . . . . . . . . . . . . . . . . . . . . . . . . . . . 11
5.4 Parametric bootstrap . . . . . . . . . . . . . . . . . . . . . . . . . . . . . . 12
5.4.1 Parameter correlations . . . . . . . . . . . . . . . . . . . . . . . . . 13
5.4.2 Sloppiness . . . . . . . . . . . . . . . . . . . . . . . . . . . . . . . . 16
5.5 Contemporary migration test . . . . . . . . . . . . . . . . . . . . . . . . . 16
5.6 Rare alleles . . . . . . . . . . . . . . . . . . . . . . . . . . . . . . . . . . . 17

**6 Settlement of New World model** 19
6.1 Alternative demographic models . . . 19
6.2 Maximum likelihood parameters . . . 20
6.3 Parametric bootstrap . . . 20
6.3.1 Parameter correlations . . . 21
6.4 Comparison with Out of Africa model parameters . . . 21
6.5 Admixture variability . . . 21
6.6 Rare alleles . . . 23

**7 Nonsynonymous variation** 28

# 1 Properties of the AFS

## 1.1 Distinguishing reduced divergence and increased migration

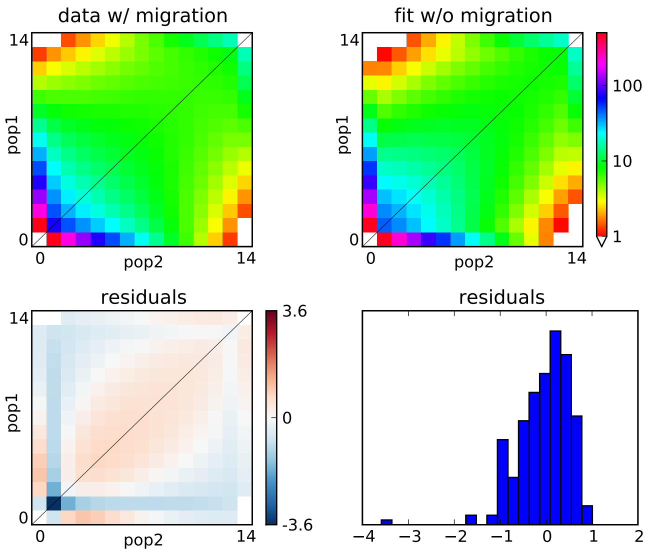


Figure 1: Fitting data including migration with a no-migration model.

As an example of inference with migration, consider the demographic scenario of Fig. MT.1 for parameter values of moderate migration and divergence: $\theta = 1000$, $\nu_1 = \nu_2 = 0.5$, $M = 2$, and $\tau = 0.3$. The noise-free AFS is shown in the upper left panel of Figure 1. For a model with $M \equiv 0$ fit to this AFS, the maximum likelihood parameters are: $\theta = 1034.4$, $\nu_1 = \nu_2 = 0.44$, and $\tau = 0.084$. As expected, when we neglect migration the inferred divergence time is substantially smaller. Less obviously, the ancestral population size (proportional to $\theta$) is overestimated, while current populations sizes are underestimated. The resulting AFS is shown in the upper right panel of Figure 1 and is qualitatively very similar

to the AFS with migration. As illustrated in the lower left panel, however, fitting this incorrect model yields correlated residuals; the model predicts too few shared polymorphisms at low frequency in one or both populations. This is the AFS signal that distinguishes between reduced divergence time and increased migration.

# 2 Numerical methods

## 2.1 Finite-difference scheme

Note: here we index populations using lower-case Greek indices, to distinguish from the numerical index we use over grid points.

To numerically approximate the solution to our diffusion equation (Eqn. MT.1) for $P$ populations, we discretize the equation over a non-uniform regular $P$-dimensional grid. (The grid is described in section 2.3). To solve this multidimensional problem, we adopt an alternating difference scheme [1], in which we evolve terms involving derivatives in each variable $x_\alpha$ separately. Here we outline the finite difference scheme we use, inspired by work of Chang and Cooper [2] on diffusion equations arising in plasma physics.

Importantly, aside from the boundary conditions our diffusive evolution conserves probability. For stability and accuracy our finite difference scheme should also explicitly conserve probability. This motivates us to consider the *fluxes* $F_\alpha$. Our diffusion equation can be decomposed into fluxes as

$$\frac{\partial \phi}{\partial \tau} = \frac{1}{2}\sum_\alpha \frac{\partial^2}{\partial^2 x_\alpha}\left(V^{(\alpha)}\phi\right) - \sum_\alpha \frac{\partial}{\partial x_\alpha}\left(M^{(\alpha)}\phi\right) \tag{1}$$

$$= \sum_\alpha \frac{\partial}{\partial x_\alpha}\left[\frac{1}{2}\frac{\partial}{\partial x}\left(V^{(\alpha)}\phi\right) - M^{(\alpha)}\phi\right] \tag{2}$$

$$= \sum_\alpha \frac{\partial}{\partial x_\alpha} F_\alpha, \tag{3}$$

where $V^{(\alpha)} = x_\alpha(1 - x_\alpha)$, and $M^{(\alpha)} = \sum_\beta M_{\alpha \leftarrow \beta}(x_\beta - x_\alpha)$.

If we take a centered finite difference about point $j$ on our grid $x_i$, where $i = 1, 2, \ldots G$, we obtain

$$\frac{\phi_j^{t+1} - \phi_j^t}{\Delta t} = \frac{1}{\Delta_j}\left(F_{j+1/2}^{t+1} - F_{j-1/2}^{t+1}\right). \tag{4}$$

To conserve total probability (as defined by the trapezoidal numerical integration scheme) we take $F_{-1/2} \equiv F_{G+1/2} \equiv 0$ and

$$\Delta_j = \begin{cases} (x_1 - x_0)/2, & j = 0, \\ (x_{i+1} - x_{i-1})/2, & 0 < j < G, \\ (x_G - x_{G-1})/2, & j = G. \end{cases} \tag{5}$$

To evaluate $F^{t+1}_{j+1/2}$, we take a centered finite-difference, so that

$$F^{t+1}_{j+1/2} \equiv \frac{1}{x_{j+1} - x_j} \frac{1}{2}\left(V_{j+1}\,\phi^{t+1}_{j+1} - V_j\,\phi^{t+1}_j\right) - M_{j+1/2}\,\phi^{t+1}_{j+1/2} \tag{6}$$

where $\phi^{t+1}_{j+1/2} \equiv \frac{1}{2}\left(\phi^{t+1}_j + \phi^{t+1}_{j+1}\right)$. (Note that Chang and Cooper take a non-centered difference on $\phi$ to ensure non-negativity of the equilibrium solution. This is not possible for us, because the equilibrium solution of our equations can be singular.)

Combining equations 4 and 6 yields a tridiagonal system of equations which can be solved by standard methods, e.g. $a_j\phi^{t+1}_{j-1} + b_j\phi^{t+1}_j + c_j\phi^{t+1}_{j+1} = \phi^t_j$.

The flux out is handled by particular absorbing terms [3] of the form:

$$\frac{\phi^{t+1}_0 - \phi^t_0}{\Delta t} = \frac{1}{\Delta_0}\left(-\frac{1}{2}\left.\frac{\partial V}{\partial x}\right|_{x=0} + M_0\right)\phi^{t+1}_0, \tag{7}$$

$$\frac{\phi^{t+1}_G - \phi^t_G}{\Delta t} = \frac{1}{\Delta_G}\left(\frac{1}{2}\left.\frac{\partial V}{\partial x}\right|_{x=1} - M_G\right)\phi^{t+1}_G. \tag{8}$$

These are applied only at the grid points where all frequencies equal 0 or 1 respectively.

New mutations are injected into the system at each timestep via:

$$\frac{\phi^{t+1}_1 - \phi^t_1}{\Delta t} = \frac{\theta}{2}\frac{1}{x_1}\frac{2^P}{(x_2 - x_0)x_1^{P-1}} \tag{9}$$

The final term (involving $2^P$) normalizes the probability density given trapezoid rule integration over the other dimensions of the grid. Note that we inject probability at a rate $\theta/(2x_1)$, independent of the relative population size $\nu_\alpha$. This reflects the fact that mutations are being input at $x_1$, not $1/(2N_\alpha)$. The effect of relative population size is accounted for by the drift term $V$.

In total, for a $P$-dimensional problem, each timestep requires solving $G^{P-1}$ tridiagonal systems of size $G$. We set our timestep to be $\Delta t \equiv \min \Delta x/10$, which provides good stability and accuracy for the scenarios considered here. (Situations with very high migration rates or selection coefficients or very small population sizes may require finer timesteps.) Thus the total run time for a single likelihood evaluation is order $G^{P+1}$.

## 2.2 Population splits

Numerically handling $\delta$-function density for $\phi$ upon population splits (Eqn. MT.2) involves some subtlety. In particular, it is important to properly conserve $\phi$ density, and the value $z$ to which a given pair of $x$ and $y$ map to may not be a point in the grid.

Consider $x$ and $y$ which map to a value $z$ which lies between grid points $z_i$ and $z_{i+1}$. Define $\Delta z_i \equiv z_{i+1} - z_i$. We distribute the density $\phi(x,y)$ which a proportion $a$ going to $z_i$ and $b$ going to $z_{i+1}$, such that

$$a = \frac{z_{i+1} - z}{\Delta z_i}, \qquad b = \frac{z - z_i}{\Delta z_i}. \tag{10}$$

To ensure proper normalization under the trapezoid rule in the interior of our domain, we must have

$$\frac{a}{2}C\Delta z_{i-1} + \frac{a+b}{2}C\Delta z_i + \frac{b}{2}C\Delta z_{i+1} = \phi(x,y). \tag{11}$$

Upon splitting, a contribution $aC$ is thus added to element $\phi(x, y, z_i)$ and a contribution $bC$ to $\phi(x, y, z_{i+1})$.

The edge cases, in which $z$, for example, maps between $z_1$ and $z_2$ are handled similarly. In those cases, Eqn. 11 must simply be altered to reflect the correct trapezoidal integration rule for those edge cases.

## 2.3 Non-uniform grid

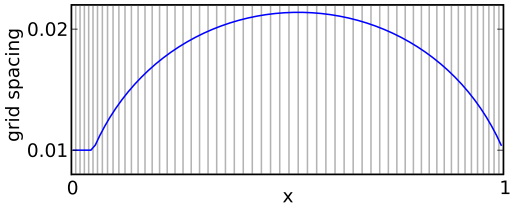


Figure 2: The nonuniform grid used in our numerical solution of the diffusion Eqn. MT.1, for $G = 60$. The vertical lines denote grid points spaced on $(0, 1)$, while the blue line traces the spacing between adjacent grid points.

We solve our equations on a non-uniform $x$ grid. For a grid of $G$ points, the first $G/10$ points (rounded down) are uniformly spaced within $x \in [0, 0.05]$. This uniform grid spacing makes the solution more accurate in the low-frequency regime, where we have many segregating mutations and the data are therefore relatively less noisy.

The remaining points are placed so that their spacings increase quadratically, being finer at small and large values of $x$. This scheme minimizes the difference in spacings between adjacent grid points, which we found helped accuracy and stability. Specifically, we take the remaining points onto $q \in [0, 1]$ which is mapped onto $x$ by $x = a\,q^3 + b\,q^2 + c\,q + d$, were $d = 0.05$, $c$ is equal to the spacing between the first $G/10$ points, $b = -3(\Delta q + c + \Delta q\,d)/\Delta q$, $a = -(2/3)b$. This pattern of grid points is illustrated in Figure 2.

Because our algorithm run time scales as $O(G^4)$ when working with 3 populations, this non-uniform grid gives a dramatic increase in computational speed for a given solution accuracy.

## 2.4 Extrapolation

Our numerical approximation to the solution of the diffusion equation improves as the grid becomes finer, as $G \to \infty$. Our computational costs, however, increase rapidly with $G$. To overcome this, we use Richardson extrapolation [1], extrapolating on the log of each entry of

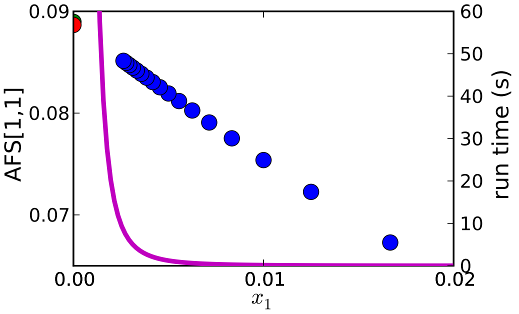


Figure 3: Extrapolation results. The blue points show the evaluation of AFS[1,1] for $G = \{40, 50, ...200\}$. The green dot is the value extrapolated from the evaluations with $G = \{40, 50, 60\}$. The red dot is the result of averaging $10^8$ simulations from `ms`. The purple line shows the run time for this two-dimensional problem as a function of grid spacing. The extrapolated evaluation took ≈0.5 seconds.

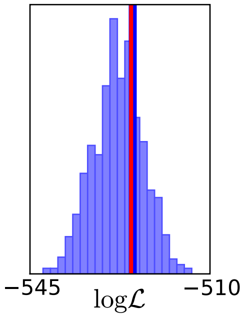


Figure 4: Diffusion-coalescent comparison for low migration. As in Figure 1.E. from the main text, but with $M = 0.1$.

the AFS, as in Eqn. MT.5. As illustrated in Figure 3, this yields a massive improvement in the accuracy of our calculated AFS. (A more sophisticated treatment of the mutation influx boundary conditions [4] may alleviate some of the bias introduced by the finite grid, but extrapolation would still enhance accuracy.)

The demographic scenario simulated in Figure 3 is as in Fig. MT.1, with $\theta = 1$, $\nu_1 = \nu_2 = 1$, $M = 1$, $T = 0.5$. The corresponding *ms* command is:

```
ms 40 1e8 -t 1 -I 2 20 20 -n 1 1 -n 2 1 -ma x 2 2 x -ej 0.25 2 1 -en 0.25 1 1
```

## 2.5 Small-$M$ comparison with *ms*

The human applications we consider here involve relatively high migration rates, so there are very few fixed differences between populations. In other cases, much smaller migration rates

may be of interest, so we have additionally compared performance between diffusion and coalescent simulations for $M = 0.1$, using the same procedure as reported in the main text for $M = 2$. Figure 4 shows that our method is again very accurate in likelihood evaluation. The speed advantage of the diffusion method is similar in this case to the $M = 2$ case.

# 3 Data processing

The 219 genes we consider yield 5,017,161 bases of non-coding sequenced DNA, with 31,352 observed SNPs in the EGP samples. Table 8 gives a gene-by-gene break down of the data.

To apply the statistical correction for ancestral misidentification [5], we align to the panTro2 build of the chimp genome using BLAT [6]. Genes longer than the 25 kb recommended for BLAT were split into 25 kb chunks with 2 kb overlap. Each 25 kb chunk was required to have at least 90% identity with chimp across at least 70% of the sequence, or it was discarded from analysis.

To apply the ancestral misidentification correction to a SNP it must satisfy 4 criteria. 1) It must have been successfully aligned to chimp. 2) The chimp allele must be one of the segregating human alleles. 3) The two bases flanking the SNP must be the same in chimp and human. 4) The SNP cannot be adjacent to any other SNP. All these criteria are satisfied for 27,824 SNPs in our sample.

## 3.1 Projection

To account for missing data and ease visual comparison between populations, we project each AFS down to 20 samples per population using a hypergeometric distribution. In essence, to project from $n$ successful calls in a population to $m$, we average over all possible results of choosing a size $m$ subsample from those $n$ calls. Because the sampling in each population is independent of sampling in the others, this is a simple extension of the one-dimensional case [7]. In particular, if we are projecting an AFS $S$ from a sample size in population $\alpha$ of $n$ to a sample size of $m$, the projected AFS $P$ is

$$P[i_\alpha, i_\beta, \ldots] = \sum_{d=i_\alpha}^{n-m+i_\alpha} \frac{\binom{m}{i_\alpha}\binom{n-m}{d-i_\alpha}}{\binom{n}{d}} S[d, i_\beta, \ldots]. \tag{12}$$

Note that this projection reduces the number of segregating SNPs, as SNPs segregating in the original sample may project to make contributions to the 'absent in the sample' and 'fixed in the sample' classes.

For our Out of Africa model, which uses YRI, CEU & CHB data, 25,258 SNPs have $\geq 20$ calls in every population. We correct our estimation of the ancestral population size for the SNPs lost to the ancestral misidentification criteria and the $\geq 20$ calls criteria by using an effective sequenced length. In this case, it is $5.02$ Mb $\cdot\, 25,259/31,352 = 4.02$ Mb. After projection, our AFS sums to 17,446 segregating SNPs.

For the New World model we have 26,387 SNPs with $\geq 20$ calls in every population, yielding an effective sequencing length of 4.20 Mb. Our projected AFS, however, contains only 13,290 segregating SNPs, reflecting lower diversity in these populations.

### 3.2 LD calculation

Fig. MT.2.D. and Fig. MT.3.D. show linkage disequilibrium as a function of physical distance in the data. These values were calculated using phased haplotypes generated using PHASE 2.0 [8] and provided by the EGP. For comparison with our simulated data, only SNPs in non-coding regions and with minor allele frequency $\geq 10\%$ in all populations were considered.

### 3.3 Estimating $\mu$

We estimate the neutral mutation rate $\mu$ using the divergence between human and chimp. Comparing aligned sequences in our data, we estimate the divergence to be 1.13%. Assuming a divergence time of 6 million years [9] and a mean generation time for human and chimp over this interval of 25 years, we have

$$\mu = 0.0113 \cdot 25/(2 \cdot 6 \times 10^6) = 2.35 \times 10^{-8} \text{ per generation.} \tag{13}$$

Note that the assumed generation time formally cancels in the conversion between genetic and chronological time units. If $t_C$ is the chronological time, $\tau$ is the genetic time (in units of $2N_A$ generations), and $t_g$ is the generation time, then

$$t_C = t_G \cdot t_g = \tau \cdot 2N_A \cdot t_g = \tau \cdot \frac{\theta}{2\mu} \cdot t_g. \tag{14}$$

As shown in the previous paragraph, $\mu$ is proportional to $t_g$, resulting in the cancellation of $t_g$.

## 4 Coalescent simulations

Detailed simulations of the EGP data are required to estimate accurate confidence intervals and to perform realistic goodness-of-fit and hypothesis tests. For these simulations, we use *ms* [10].

To account for potential linkage between genes, in our simulations we divide the 219 sequenced genes into 194 potentially linked regions, each separated by at least 500 kb (Table 8). We simulate the entirety of each region using a value for $\theta$ scaled by the relative length of that region to the total sequenced length. The recombination rate for each region is set to the average recombination rate from the HapMap Release 22 genetic map [11]. This rate $r$ was converted into a population-scaled rate $\rho = 2N_{ref}r$ by using $N_{ref}$ inferred from $\theta$ and our estimate of $\mu$.

Simulations use the total number of samples from each EGP population. The resulting AFS is then projected down to 20 samples per population. When extracting an AFS from a simulation, only SNPs lying within regions sequenced by the EGP are included.

### 4.1 Reduction of effective independent SNPs by linkage

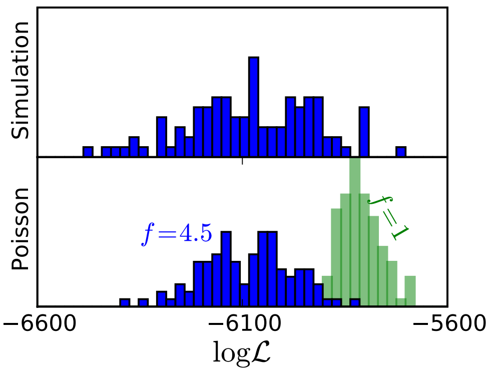


Figure 5: Shown are histograms of the likelihoods of generated data sets under the model. Data sets in the top panel are simulated using the coalescent procedure described above. Data sets in the bottom panel are simulated using the modified Poisson procedure described below, where the effective number of data points has been reduced by a factor $f$.

To first order, the effect of linkage on our analysis is to reduce the effective number of independent samples in the frequency spectrum. To estimate the magnitude of this effect, in Figure 5 we compare the distribution of likelihoods generated by the full simulation procedure described above and by modified Poisson sampling from the model frequency spectrum $M$. In the modified Poisson sampling, we sample from $M/f$ and then multiply the resulting sampled frequency spectrum by $f$. In effect, this generates a frequency spectrum where each sample is replicated $f$ times.

As illustrated in Figure 5, the likelihood distributions are similar for $f = 4.5$. This suggests that linkage reduces the effective number of independent samples in our data by a factor of approximately 4.5. Note that the likelihood distribution for the full simulations remains somewhat wider than that for $f = 4.5$, indicating that the effect of the linkage in the data is more than a simple consistent reduction in the number of effective data points.

# 5 Out of Africa model

## 5.1 Marginal analyses

Figure 6 and Table 1 present results from a two-epoch model fit to the YRI spectrum. The fit is quite good, and the inferred parameter values are reasonable and consistent with estimates from other studies.

Figure 7 and Table 2 present results from a divergence and growth model fit to the CEU/CHB spectrum. (In this model both populations diverge from an equilibrium population and grow exponentially following a concurrent bottleneck.) Here we do see a pattern of

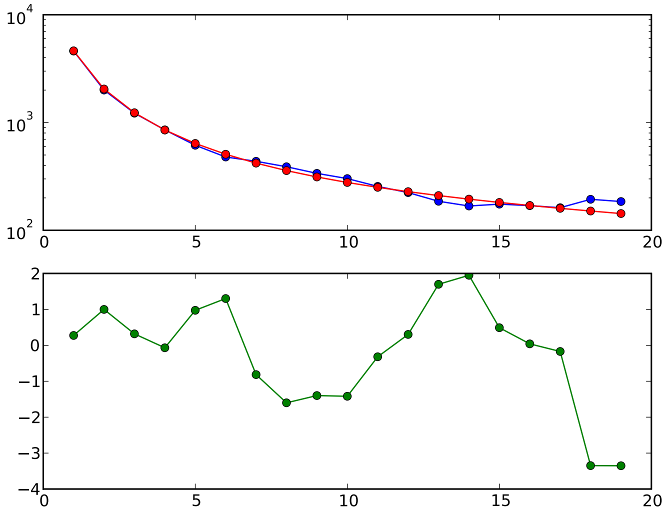


Figure 6: YRI marginal fit. The top panel shows the model (red) and data (blue) spectra. The bottom panel shows the residuals.

Table 1: Maximum-likelihood parameters for YRI marginal fit.

| parameter | value |
|---|---|
| $N_A$ | 7,100 |
| $N_{AF}$ | 13,600 |
| $T_{AF}$ (kya) | 136 |

correlated residuals, in that the model underestimates the amount of high frequency shared polymorphism. As seen in Fig. MT.2, the more complex model which incorporates migration from YRI alleviates this somewhat. Allowing the bottleneck times in the two populations to occur anytime after divergence yielded only a very slight increase in fit quality (data not shown).

## 5.2 Maximum likelihood parameters

In genetic units (scaled by $N_A$), the maximum likelihood parameters are shown in Table 3. In *ms* syntax, the demographic model is:

```
-n 1 1.682020 -n 2 3.736830 -n 3 7.292050
-eg 0 2 116.010723 -eg 0 3 160.246047
-ma x 0.881098 0.561966 0.881098 x 2.797460 0.561966 2.797460 x
-ej 0.028985 3 2 -en 0.028985 2 0.287184
-ema 0.028985 3 x 7.293140 x 7.293140 x x x x x
-ej 0.197963 2 1 -en 0.303501 1 1'
```

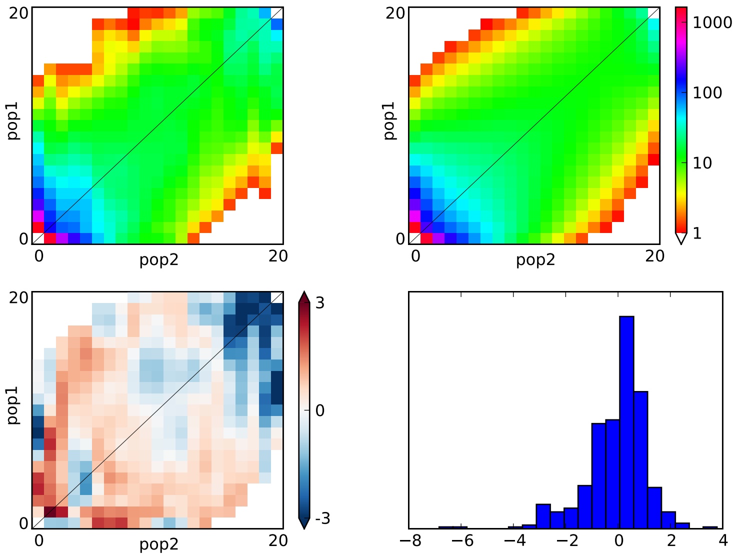


Figure 7: CEU/CHB marginal fit. The upper left panel shows the data, and the upper right the model. The lower panels show the residuals, as a heat map and as a histogram.

Table 2: Maximum-likelihood parameters for CEU/CHB marginal fit.

| parameter | value |
|---:|---|
| $N_A$ | 6,650 |
| $N_{EU0}$ | 1,730 |
| $N_{EU}$ | 20,000 |
| $N_{AS0}$ | 330 |
| $N_{AS}$ | 35,000 |
| $m_{EU-AS}$ ($\times 10^{-5}$) | 34 |
| $T_{EU-AS}$ (kya) | 18.4 |

To convert to physical units, we use $\theta = 4N_A \mu L$, where $L$ is the length of sequence considered. Importantly, $L$ must use the effective sequenced length, which accounts for losses in alignment and missed calls. So

$$N_{ref} = \frac{\theta}{4L\mu} = \frac{2788.2}{4 \cdot 4.04 \times 10^6 \cdot 2.35 \times 10^{-8}} = 7310. \tag{15}$$

The remaining conversions are straightforward.

## 5.3 Projection and residuals

Some the correlation between residuals seen in Fig. MT.2 and MT.3 is due to the fact that we've projected the data down from a larger sample size. This effect is illustrated in

Table 3: Maximum likelihood parameter values for Out of Africa model, in genetic units.

| parameter | value | parameter | value |
|---|---|---|---|
| $\theta_T$ | 2788.2 | $M_{AF-B}$ | 3.65 |
| $\nu_{AF}$ | 1.68 | $M_{AF-EU}$ | 0.44 |
| $\nu_B$ | 0.287 | $M_{AF-AS}$ | 0.28 |
| $\nu_{EU0}$ | 0.129 | $M_{EU-AS}$ | 1.40 |
| $\nu_{EU}$ | 3.74 | $T_{AF}$ | 0.607 |
| $\nu_{AS0}$ | 0.070 | $T_B$ | 0.396 |
| $\nu_{AS}$ | 7.29 | $T_{EU-AS}$ | 0.058 |

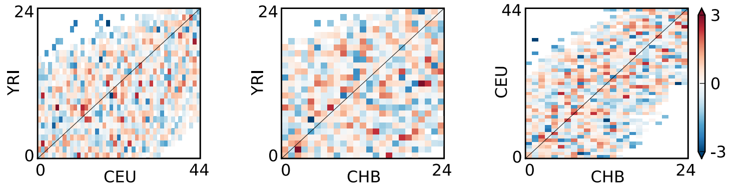

(a) Model comparison with sampled spectrum

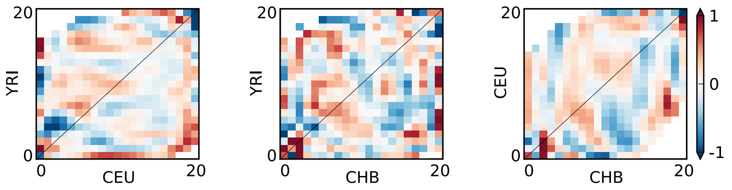

(b) Model comparison with projected spectrum

Figure 8: Effect of projection on residuals. As shown in (b), projecting a data set down from a larger sample size yields correlated 'splotchy' residuals.

Figure 8. In subfigure (a) we show the residuals between our model AFS simulated for the total number of individuals in the EGP and a Poisson sampling from that AFS. As expected, the residuals shown no correlation. Subfigure (b) compares the model AFS with the same sampled AFS as in (a), but projected down to 20 samples per population. This projection results in correlation between adjacent entries in the AFS that is very similar to that seen in the model comparison with the real data.

## 5.4 Parametric bootstrap

Shown in Figure 9 are the results of the parametric bootstrap analysis of parameter uncertainties for our Out of Africa model. All distributions of bootstrap parameter estimates have their mode approximately at the maximum likelihood value. This provides empirical evidence that, as expected, our estimation is not significantly biased.

### 5.4.1 Parameter correlations

The correlations between parameter values inferred during our conventional bootstrap shed light on the dependencies between model parameters. Figure 10 shows the squared correlation coefficient between each of the inferred parameter values. Correlations are typically low, with a few exceptions.

Figure 11 illustrates three of the most strongly correlated parameter pairs. The strongest correlation is between the time of the African population size change $T_{AF}$ and the ancestral population size $N_A$. This likely reflects the need to generate the appropriate level of polymorphism before divergence from Africa. Interestingly, the divergence time between CEU and CHB, $T_{EU-AS}$, is more strongly correlated with the growth rate of the Asian population $r_{AS}$ than with the migration rate between the two populations $m_{EU-AS}$.

The lower-right panel of Figure 11 compares inferred values of the initial population sizes for European and Asian populations, $N_{EU0}$ and $N_{AS0}$, respectively. There is little correlation between the inferred values. 92 of our 100 bootstrap fits yield $N_{EU0} > N_{AS0}$.

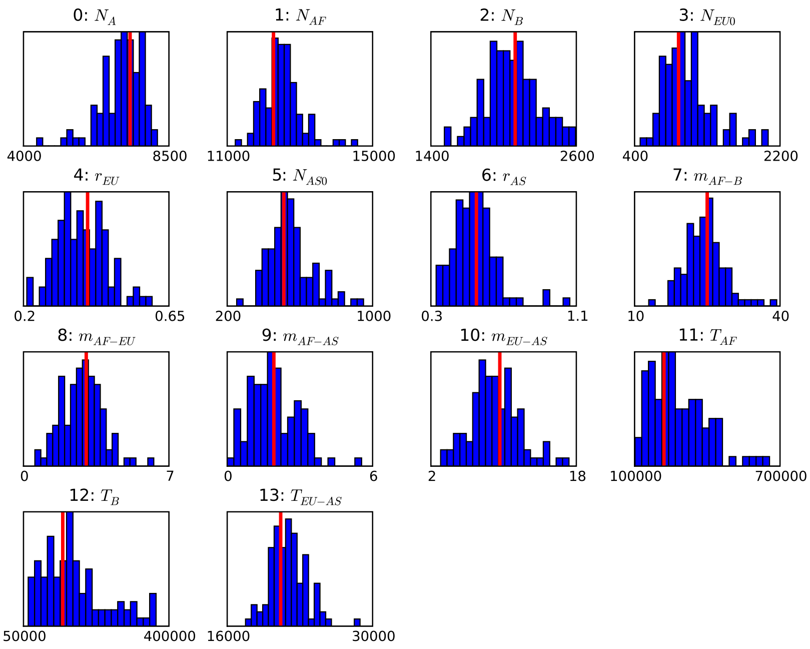


(a)

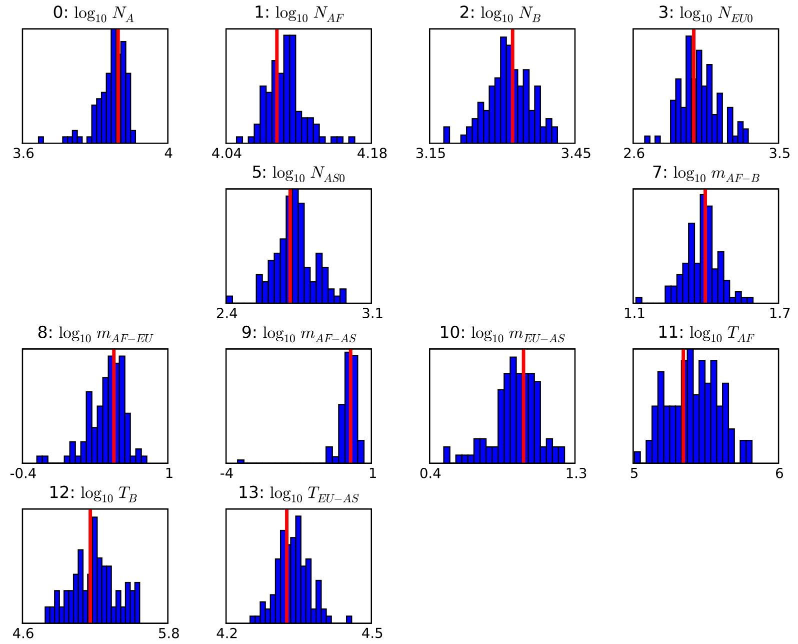


(b)

Figure 9: Out of Africa model parametric bootstrap results. Shown the results of fits to 100 simulated data sets, generated using maximum likelihood values from the real data (red lines). For parameters defined to be positive, also shown are the logarithms of the bootstrap results, as these were used in confidence interval calculations. Particularly for $T_{AF}$ and $T_B$, they are much closer to normally distributed.

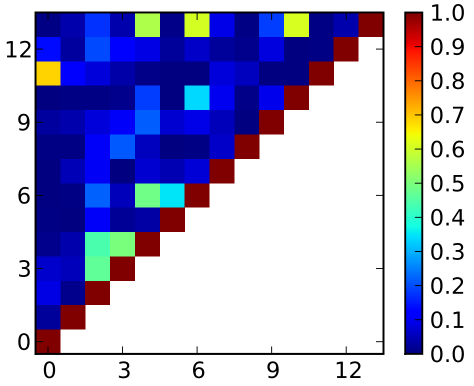


Figure 10: Correlation ($r^2$) between bootstrap parameter values for Out of Africa analysis. Parameter indices are as in Figure 9.

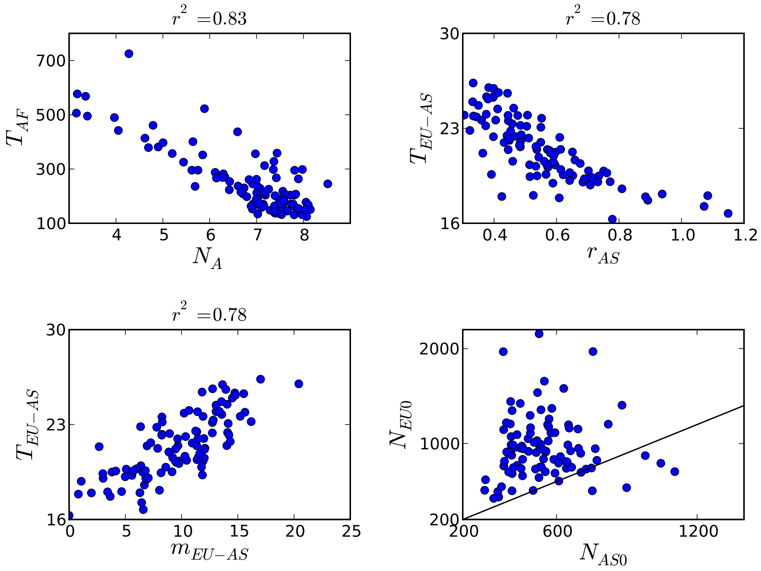


Figure 11: The first three panels are the highly correlated pairs of parameters in our Out of Africa analysis. ($N_A$ and $T_{EU-AS}$ have been divided by 1000 for plotting, and $m_{EU-AS}$ has been multiplied by $10^5$.) The line in the lower right panel is $N_{EU0} = N_{AS0}$.

### 5.4.2 Sloppiness

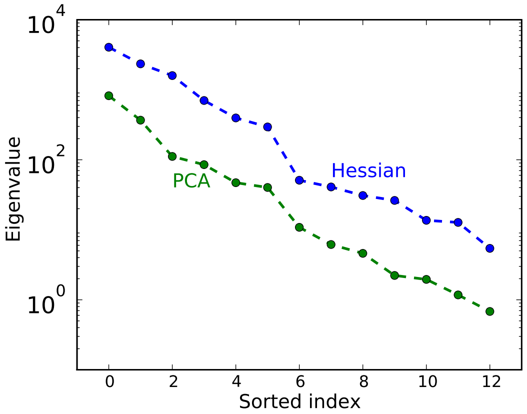


Figure 12: Plotted are the eigenvalues of the model Hessian matrix and a Principle-Components-Analysis of our 100 parametric bootstrap parameter sets. The fact that these plots are roughly straight lines indicates that the model is 'sloppy'.

Recently it has been suggested that the sensitivities of many-parameter models to changes in those parameter values follow a universal 'sloppy' distribution [12]. This distribution is characterized by eigenvalues of the Hessian matrix $(\partial^2\mathcal{L}/\partial \log p_i \partial \log p_j)$ which decrease linearly in their logarithm. As illustrated in Figure 12, the demographic model we fit exhibits a sloppy spectrum of sensitivities. As expected, a principle components analysis of our ensemble of 100 parameter sets derived from fitting simulated data sets shows a similar sloppy pattern.

The sloppiness we see is indicative of strong correlations between the effects of different parameters on the AFS. In some problems, it is possible to define an orthogonal parameterization which eliminates these correlations [12]. Such a parameterization has been demonstrated for the single-population AFS [13], but none is know yet for the multiple-population case.

Additionally, the fact that this model is sloppy is interesting because the model was designed to be parsimonious, and in all previous examples of sloppy systems the parameterization was determined by biological or physical considerations. This example expands the domain of 'sloppy' problems.

## 5.5 Contemporary migration test

Fitting the data with a model lacking contemporary migration yields the parameters in Table 4. In our test, we generate simulated data sets with these parameters, then fit them with a model allowing contemporary migration.

Table 4: Maximum likelihood parameter values for Out of Africa model without contemporary migration, in genetic units.

| parameter | value | parameter | value |
|---|---|---|---|
| $\theta_T$ | 2532.4 | $M_{AF-B}$ | 3.65 |
| $\nu_{AF}$ | 1.82 | | |
| $\nu_B$ | 0.319 | | |
| $\nu_{EU0}$ | 0.149 | | |
| $\nu_{EU}$ | 8.41 | $T_{AF}$ | 1.28 |
| $\nu_{AS0}$ | 0.066 | $T_B$ | 0.897 |
| $\nu_{AS}$ | 34.36 | $T_{EU-AS}$ | 0.052 |

## 5.6 Rare alleles

In Figure 2.E. of the main text, we evaluate the goodness-of-fit of our model to the observed data using our composite likelihood function. This function involves the entirety of the frequency spectrum, and in some cases specific frequency classes may be of particular interest. In particular, rare alleles may be of medical interest. Table 5 compares our the rare-allele entries of our bootstrap simulations with the real data. Each entry in the tables records the fraction of bootstrap simulations which yielded a larger proportion of SNP in that entry that in the real data. For example, 3% of simulations yield a larger proportion of SNPs that are at frequency (2,1,1) in (YRI,CEU,CHB) samples, respectively, than is observed in the real data. In general, the proportions seen in the real data are typical in our simulations. For some entries the real data may be atypical of the simulations, but it is unclear whether these deviations are signficant.

Table 5: P-values of rare frequency spectrum entries. The tables record the fraction of parametric bootstrap simulations yielding larger proportion of mutations in a given frequency class than observed in the data.

| CEU | | | | |
|---|---|---|---|---|
| 2 | 0.45 | 0.24 | 0.34 | |
| 1 | 0.87 | 0.77 | 0.93 | |
| 0 | — | 0.68 | 0.35 | |
| | 0 | 1 | 2 | CHB |

(a) Sample YRI frequency 0

| CEU | | | | |
|---|---|---|---|---|
| 2 | 0.38 | 0.22 | 0.49 | |
| 1 | 0.41 | 0.05 | 0.63 | |
| 0 | 0.17 | 0.82 | 0.63 | |
| | 0 | 1 | 2 | CHB |

(b) Sample YRI frequency 1

| CEU | | | | |
|---|---|---|---|---|
| 2 | 0.51 | 0.05 | 0.28 | |
| 1 | 0.11 | 0.03 | 0.01 | |
| 0 | 0.65 | 0.50 | 0.13 | |
| | 0 | 1 | 2 | CHB |

(c) Sample YRI frequency 2

# 6 Settlement of New World model

## 6.1 Alternative demographic models

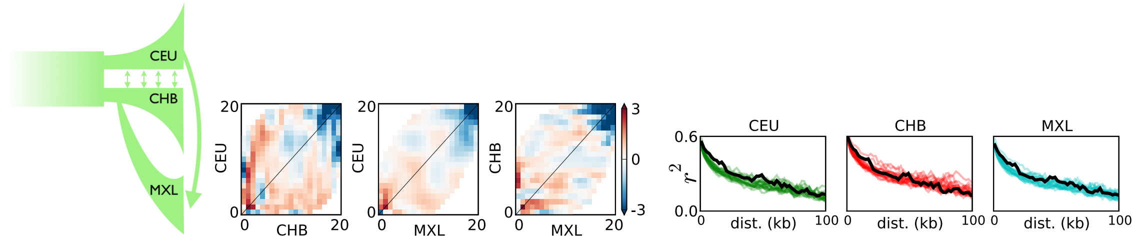


(a) Divergence from equilibrium population. $\log \mathcal{L} = -5405.9$, 11 free parameters

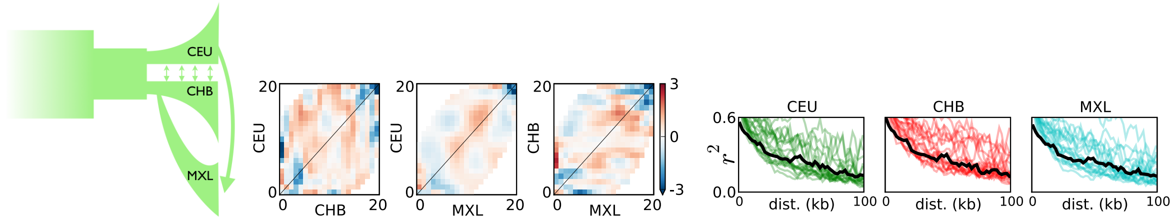


(b) Divergence from two-epoch population. $\log \mathcal{L} = -5261.8$, 13 free parameters

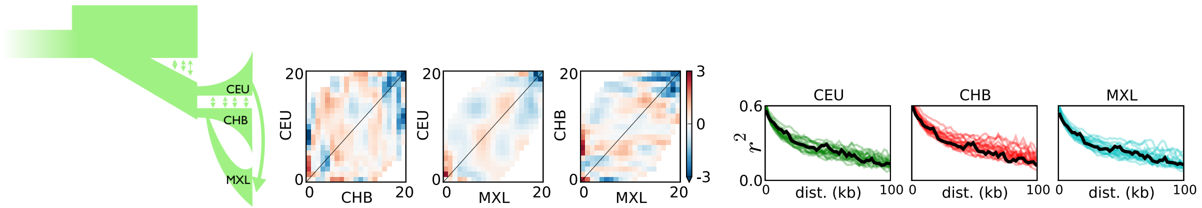


(c) With African population. $\log \mathcal{L} = -5262.0$, 10 free parameters

Figure 13: Alternative models for joint CEU,CHB,MXL demographic history. Each panel shows one of the three models we considered for modeling settlement of the New World, which differ only in history prior to the MXL divergence. Each panel also shows the residuals from the fit to the data, along with a comparison of LD decay from the real data and from the simulations.

Figure 13 illustrates several alternative demographic models considered for the Settlement of the New World. In Model (a) the CEU and CHB populations diverge from an equilibrium neutral population. Unsurprisingly, this model fails to reproduce the observed frequency spectrum well (log-likelihood = -5405.9, 11 free parameters). As an alternative, we considered Model (b), which allows for a population size change before divergence. (We allowed for the population to increase or decrease. The optimization resulting in a decrease.) This model reproduces the frequency spectrum substantially better (log-likelihood = -5261.1, 13 free parameters), but the predicted pattern of linkage disequilibrium is very different from the observed pattern. The model we settled upon is Model (c), in which the population history

Table 6: Maximum likelihood parameter values for Settlement of the New World model, in genetic units.

| parameter | value | parameter | value |
|---|---|---|---|
| $\nu_{EU0}$ | 0.208 | $M_{EU-AS}$ | 1.98 |
| $\nu_{EU}$ | 2.42 | $T_{EU-AS}$ | 0.072 |
| $\nu_{AS0}$ | 0.081 | $T_{MX}$ | 0.059 |
| $\nu_{AS}$ | 4.186 | $f_{MX}$ | 0.48 |
| $\nu_{MX0}$ | 0.103 | | |
| $\nu_{MX}$ | 7.94 | | |

prior to CEU/CHB divergence is set to the maximum likelihood history from our previous Out of Africa analysis. Note that $\theta$ must be scaled to reflect the differing effective sequence length. This model reproduces the frequency spectrum as well as Model (b) (log-likelihood = -5262.0, 10 free parameters), and it yields the correct pattern of linkage disequilibrium.

## 6.2 Maximum likelihood parameters

Table 6 gives the maximum likelihood parameter values for our Settlement of the New World. The corresponding *ms* demography is:

```
-n 1 1.682020 -n 2 2.424020 -n 3 4.185850 -n 4 7.942130
-es 0 4 0.522451 -ej 0 5 2
-eg 0 2 67.978337 -eg 0 3 109.406463 -eg 0 4 147.474095
-ema 0 5 x 0 0 0 x 0 x 3.960400 0 x 0 3.960400 x 0 x 0 0 0 x x x x x x x
-ej 0.029475 4 3
-ema 0.029475 5 x 0.881098 0.561966 x x 0.881098 x 3.960400 x x 0.561966
3.960400 x x x x x x x x x x x x x
-ej 0.036114 3 2 -en 0.036114 2 0.287184
-ema 0.036114 5 x 7.293140 x x x 7.293140 x x x x x x x x x x x x x x x
x x x
-ej 0.197963 2 1 -en 0.303500 1 1
```

Note that this command is complicated by the need to model admixture in MXL by generating a 5th population that exists for 0 time.

## 6.3 Parametric bootstrap

The parametric bootstrap results for our New World model are shown in Figure 14. Note that there does appear to be some slight bias in our inference of the growth rate, $r_{MX}$, of the MXL population. This is because our calculation of the frequency spectrum is slightly biased in evaluation of the number of singletons private to MXL. Increasing the number of grid points $G$ used in the evaluation would help eliminate this bias, at the cost of an increase in computation time.

### 6.3.1 Parameter correlations

Figure 15 shows the correlation between conventional bootstrap values between pairs of parameters.

Figure 16 plots the three most correlated parameter combinations. The correlation between MXL initial population size $N_{MX0}$ and growth rate $r_{MX}$ is particular strong. These likely represent combinations of parameters with generate the appropriate YRI and CHB divergence.

## 6.4 Comparison with Out of Africa model parameters

For those inferred parameter values that are shared between our Out of Africa and Settlement of the New World Model analyses, Figure 17 compares the distributions of conventional bootstrap estimates. Importantly, all confidence intervals overlap substantially.

## 6.5 Admixture variability

Individuals in admixed populations mary vary considerably in their ancestry. In particular, previous analyses of Mexican-Americans have found a wide range of ancestry [14]. Our model adopts a single population-level admixture proportion, and it is important that we understand the degree to varying individual ancestry affects our results.

To roughly estimate individual ancestry proportions, we adopt a maximum-likelihood approach [15] similar to the Bayesian approach used in *structure* [16]. We consider only the European and East Asian ancestry of Mexican individuals, in order to compare with our three-population simulations. This is a rather crude approximation to the possibly very complex ancestry of these individuals, but it nevertheless provides useful guidance for our simulations.

Define $q_i$ to be European ancestry proportion of Mexican individual $i$. In this rough analysis, $1-q_i$ is then that individual's East Asian ancestry proportion. For that individual, the probability of the observing the pair of alleles $x_l = (\alpha, \beta)$ at locus $l$ is:

$$P\big(x_l = (\alpha,\beta)\big) = 2\big(\mathcal{E}_{l\alpha} q_i + \mathcal{A}_{l\alpha}(1-q_i)\big)\big(\mathcal{E}_{l\beta} q_i + \mathcal{A}_{l\beta}(1-q_i)\big). \tag{16}$$

Here $\mathcal{E}_{l\alpha}$ is the frequency of allele $\alpha$ at locus $l$ in the European population. Similarly, $\mathcal{A}_{l\alpha}$ is the frequency of allele $\alpha$ at locus $l$ in the East Asian population. We simply estimate $\mathcal{E}_{l\alpha}$ and $\mathcal{A}_{l\alpha}$ by the frequencies in our CEU and CHB samples, respectively. To estimate the ancestry proportions $q_i$, we maximize the composite likelihood formed by multiplying the probability in Equation 16 over all loci.

The histogram in Figure 18 shows the European admixture proportions inferred for the 22 individuals in our Mexican-American sample. The green curve shows the distribution of admixture proportions inferred from parametric bootstrap simulations of our demographic model. These simulations were performed with $f_{MX} = 0.47$, indicated by the dashed green line. As expected, we see that our admixture inference procedure overestimates the CEU

contribution, because we have no Native American samples. Also, we see that the distribution of ancestry proportions arising from our simulations is narrower than seen in the real data. In particular, there are a few individuals in the data with unusually little European ancestry.

To roughly approximate the distribution of ancestry seen in the data, we perform simulations in which 3 of our 22 individuals have 5% European ancestry, 16 have 47%, and 3 have 60%. [1] The resulting distribution of inferred ancestries is shown by the red curve in Figure 18. This distribution captures the individuals with low-European ancestry in the real data, and is overall perhaps somewhat wider.

To test our method in the presence of an extremely wide distribution of individual ancestry, we consider a scenario in which we have 1 individual each of European ancestry proportion {0, 5%, 10% ...}. To have 22 individuals as in our data, we simulate with two individuals of European ancestry proportion 50%.[2] The resulting distribution of inferred ancestries is shown by the cyan curve in Figure 18. As expected, the distribution of inferred ancestry proportions is very wide.

We fit our CEU/CHB/MXL model to 100 data sets each simulated with our two distribution of MXL ancestry. Figure 19 compares the resulting parametric bootstrap parameter distributions with those from our single-ancestry-proportion simulations. The differences in $f_{MX}$ are expected and correctly reflect the average ancestry of individuals in each simulation. Agreement between the distributions is outstanding. Our demographic inferences are very robust to a distribution of ancestry in the MXL individuals. Remarkably, variable ancestry

---

[1] In *ms* parlance, the demograhpic history used was: `-I 6 0 44 24 6 32 6 -n 1 1.682020 -n 2 2.424020 -n 3 4.185850 -n 4 7.942130 -es 0 4 0.950000 -es 0 5 0.530000 -es 0 6 0.400000 -ej 0 9 2 -ej 0 8 2 -ej 0 7 2 -ej 0 5 4 -ej 0 6 4 -eg 0 2 67.978337 -eg 0 3 109.406463 -eg 0 4 147.474095 -ema 0 9 x 0 0 0 x x x x x 0 x 3.9604 0 x x x x x 0 3.9604 x 0 x x x x x 0 0 0 x x x x x x x x x x x x x x x x x x x x x x x x x x x x x x x x x x x x x x x x x x x x x x x x x x x x -ej 0.029475 4 3 -ema 0.029475 9 x 0.881098 0.561966 x x x x x x 0.881098 x 3.9604 x x x x x x 0.561966 3.9604 x x x x x x x x x x x x x x x x x x x x x x x x x x x x x x x x x x x x x x x x x x x x x x x x x x x x x x x x x x x x x -ej 0.036114 3 2 -en 0.036114 2 0.287184 -ema 0.036114 9 x 7.29314 x x x x x x x 7.29314 x x x x x x x x x x x x x x x x x x x x x x x x x x x x x x x x x x x x x x x x x x x x x x x x x x x x x x x x x x x x x x x x x x x x x x x -ej 0.197963 2 1 -en 0.303500 1 1`.

[2] The ms command terms handling this admixture distribution are `-I 24 0 44 24 2 2 2 2 2 2 2 2 2 2 4 2 2 2 2 2 2 2 2 2 2 -n 1 1.682020 -n 2 2.424020 -n 3 4.185850 -n 4 7.942130 -es 0 4 1.000000 -es 0 5 0.950000 -es 0 6 0.900000 -es 0 7 0.850000 -es 0 8 0.800000 -es 0 9 0.750000 -es 0 10 0.700000 -es 0 11 0.650000 -es 0 12 0.600000 -es 0 13 0.550000 -es 0 14 0.500000 -es 0 15 0.450000 -es 0 16 0.400000 -es 0 17 0.350000 -es 0 18 0.300000 -es 0 19 0.250000 -es 0 20 0.200000 -es 0 21 0.150000 -es 0 22 0.100000 -es 0 23 0.050000 -es 0 24 0.000000 -ej 0 45 2 -ej 0 44 2 -ej 0 43 2 -ej 0 42 2 -ej 0 41 2 -ej 0 40 2 -ej 0 39 2 -ej 0 38 2 -ej 0 37 2 -ej 0 36 2 -ej 0 35 2 -ej 0 34 2 -ej 0 33 2 -ej 0 32 2 -ej 0 31 2 -ej 0 30 2 -ej 0 29 2 -ej 0 28 2 -ej 0 27 2 -ej 0 26 2 -ej 0 25 2 -ej 0 5 4 -ej 0 6 4 -ej 0 7 4 -ej 0 8 4 -ej 0 9 4 -ej 0 10 4 -ej 0 11 4 -ej 0 12 4 -ej 0 13 4 -ej 0 14 4 -ej 0 15 4 -ej 0 16 4 -ej 0 17 4 -ej 0 18 4 -ej 0 19 4 -ej 0 20 4 -ej 0 21 4 -ej 0 22 4 -ej 0 23 4 -ej 0 24 4`.

Table 7: P-values of rare frequency spectrum entries. The tables record the fraction of parametric bootstrap simulations yielding larger proportion of mutations in a given frequency class than observed in the data.

| CHB | | | | |
|---|---|---|---|---|
| 2 | 0.13 | 0.32 | 0.63 | |
| 1 | 0.75 | 0.11 | 0.45 | |
| 0 | — | 0.02 | 0.59 | |
| | 0 | 1 | 2 | MXL |

(a) Sample CEU frequency 0

| CHB | | | | |
|---|---|---|---|---|
| 2 | 0.79 | 0.62 | 0.61 | |
| 1 | 0.95 | 0.84 | 0.26 | |
| 0 | 1.00 | 0.77 | 0.65 | |
| | 0 | 1 | 2 | MXL |

(b) Sample CEU frequency 1

| CHB | | | | |
|---|---|---|---|---|
| 2 | 0.38 | 0.32 | 0.61 | |
| 1 | 0.90 | 0.52 | 0.04 | |
| 0 | 0.94 | 1.00 | 0.94 | |
| | 0 | 1 | 2 | MXL |

(c) Sample CEU frequency 2

does not even effect our power, as evidenced by the fact that the widths of all the parameter distributions are identical.

## 6.6 Rare alleles

As in section 5.6, it may be of interest specifically how well our model including MXL reproduces the distribution of shared rare alleles. Table 7. In this case, it appears that our model may be somewhat overestimating the proportion of alleles that are observed to be absent or at very low frequency in CHB.

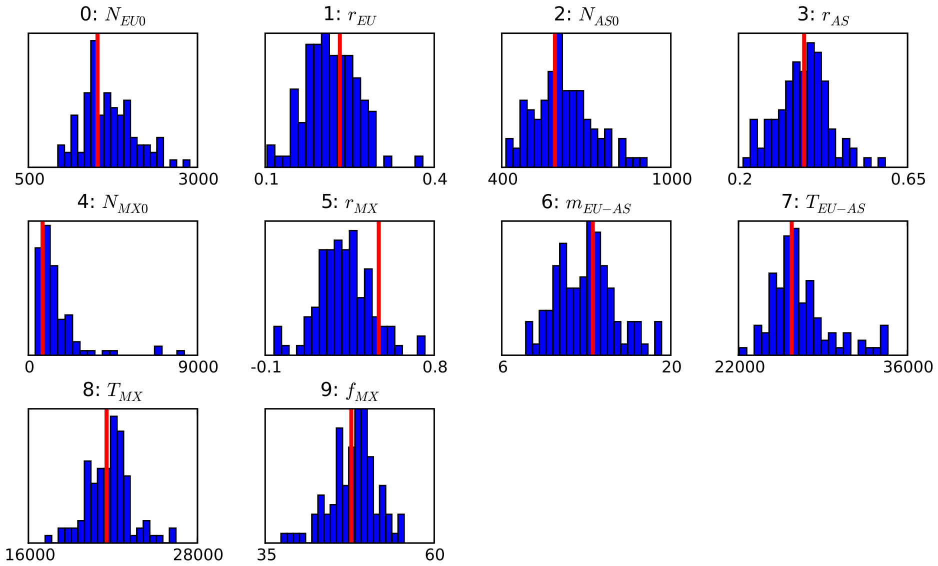


(a)

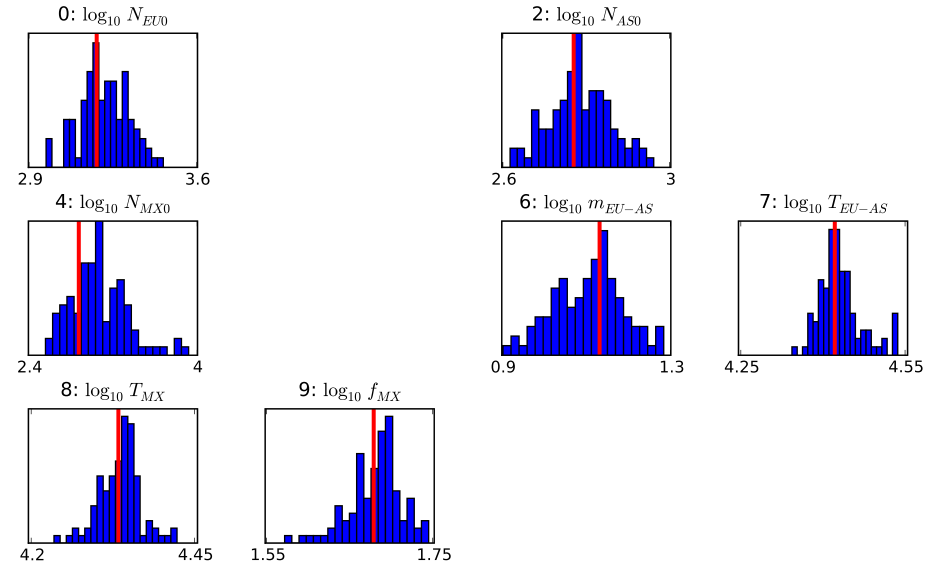


(b)

Figure 14: Settlement of New World model parametric bootstrap results.

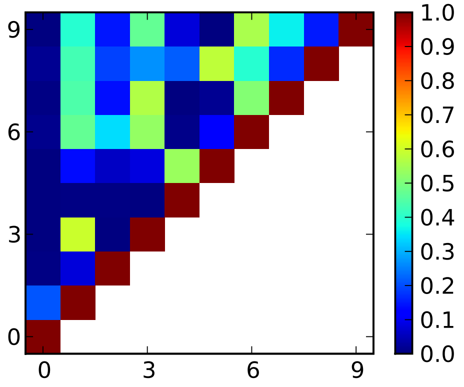


Figure 15: Correlation ($r^2$) between bootstrap parameter values for Settlement of New World analysis. Parameters are indexed as in Figure 14.

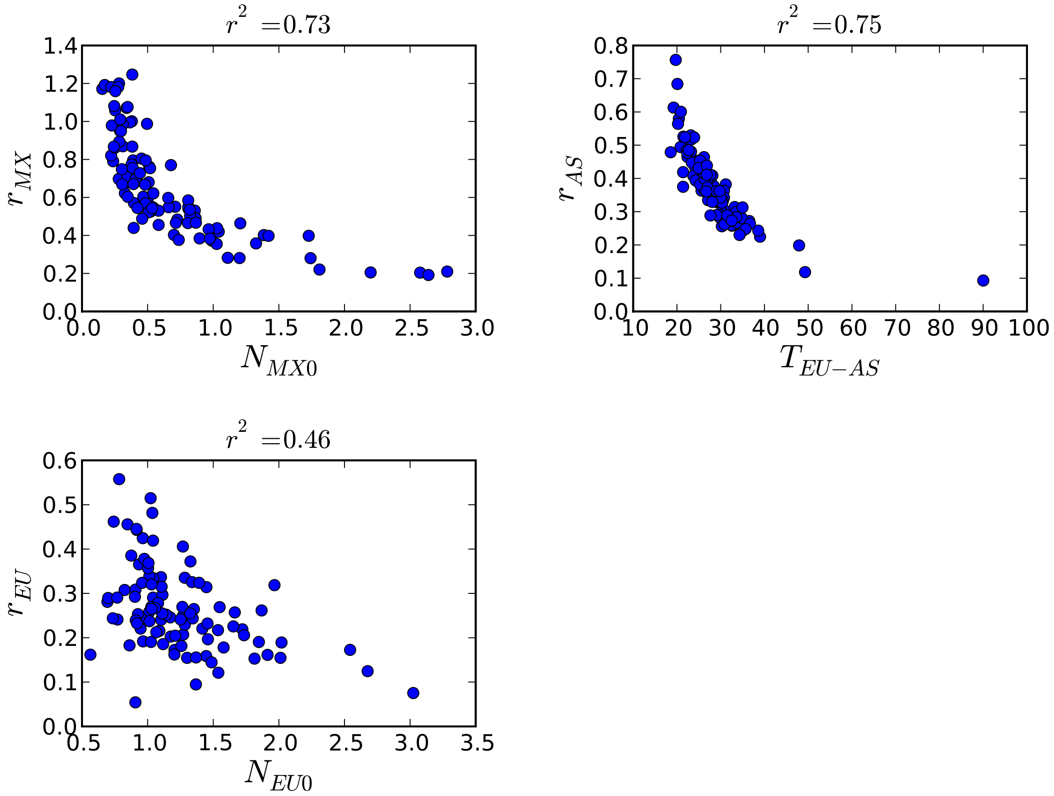


Figure 16: Plotted are conventional bootstrap values of the three most correlated parameter pairs. (For plotting $N_{MX0}$, $T_{EU-AS}$ and $N_{EU0}$ have been divided by one thousand.)

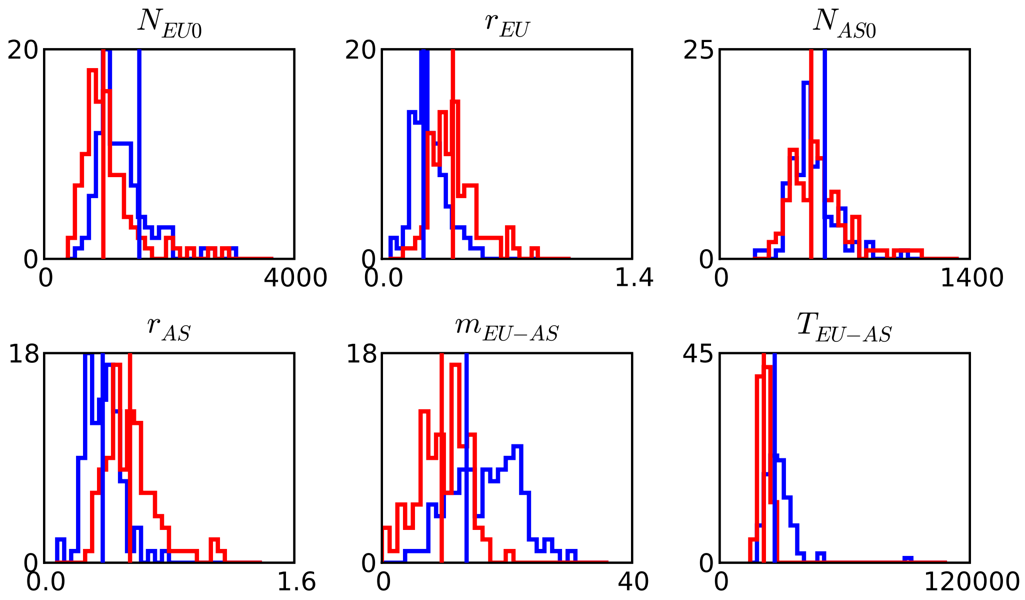


Figure 17: Comparison of parameter inferences in Out of Africa and New World models. The New World values are in blue, while the Out of Africa are red. The maximum-likelihood values are indicated by vertical lines.

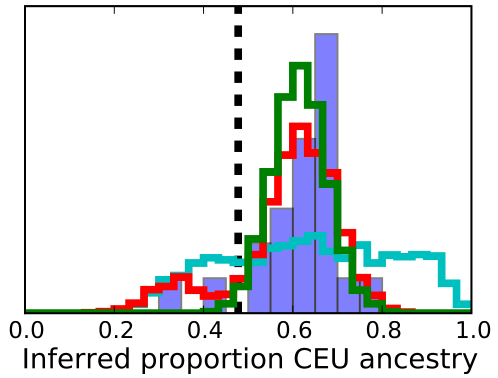


Figure 18: Distribution of inferred European ancestry proportion for real data, and simulations with varying degrees of individual ancestry variability. Histogram is the real data. The green, red, and cyan curves are, respectively, simulations with only a single admixture proportion, with a simple distribution of admixture proportions chosen to mimic the real data, and with an extremely wide distribution. Note that these are only crude estimates of European ancestry proportion, because our data lack Native American samples. This is emphasized by the dashed black line, which shows the European admixture proportion used in the single proportion simulations.

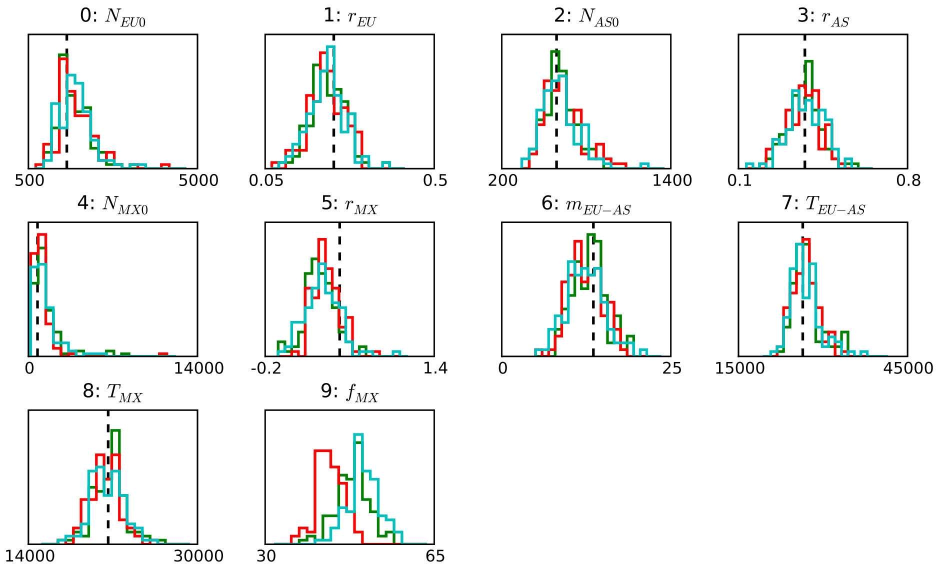


Figure 19: Comparison of parametric bootstrap results with and without variable MXL ancestry. Black dashed lines indicate parameter values used in the simulations. The blue curve shows parametric bootstrap results for simulations with only a single Mexican admixture proportion. The red curve shows parametric bootstrap results with a distribution of Mexican admixture proportions chosen to mimic that seen in the data (see Figure 18). The cyan curve results from an extremely wide distribution of ancestries. The excellent agreement between the distributions suggests that our inference procedure is very robust to variable ancestry in Mexican-American individuals.

# 7 Nonsynonymous variation

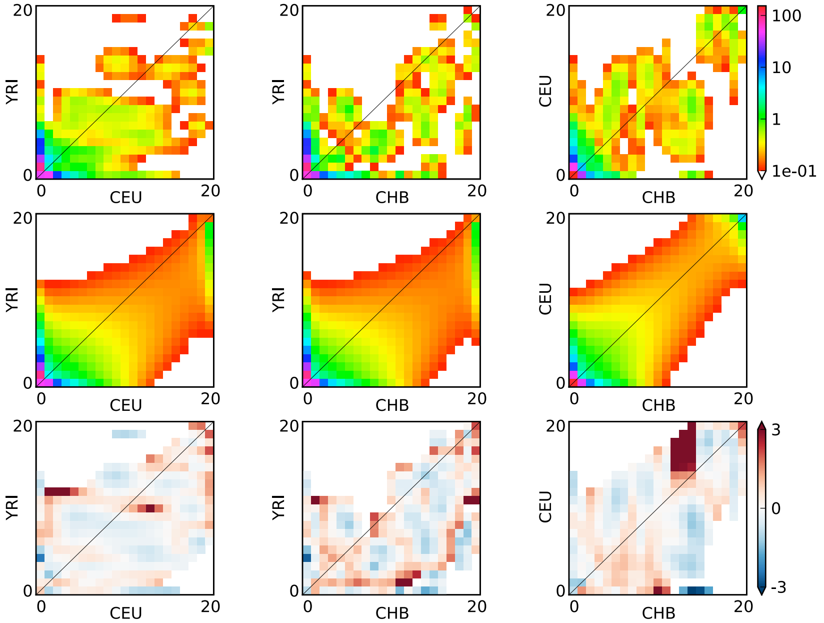


(a)

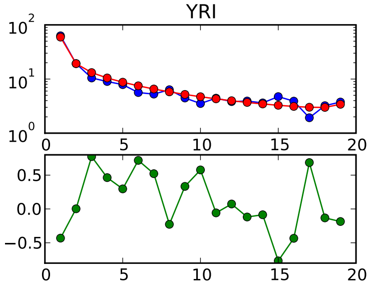


(b)

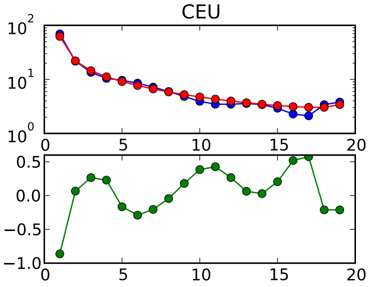


(c)

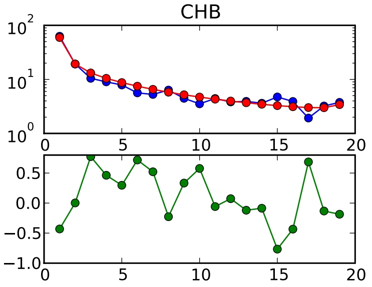


(d)

Figure 20: Detailed nonsynonymous SNP comparison. Showed are comparisons of the two- and one- dimensional marginal spectra from the data with the model. Agreement is overall reasonable, although the data is too sparse for quantitative comparison of the entire AFS.

# References

[1] Press WH, Teukolsky SA, Vetterling WT, Flannery BP (2007) Numerical Recipes: The Art of Scientific Computing. Cambridge University Press, 3rd edition.

[2] Chang JS, Cooper G (1970) A practical difference scheme for Fokker-Planck equations. J Comput Phys 6: 1–16.

[3] Kimura M (1964) Diffusion models in population genetics. J Appl Probab 1: 177–232.

[4] Evans SN, Shvets Y, Slatkin M (2007) Non-equilibrium theory of the allele frequency spectrum. Theor Popul Biol 71: 109–119.

[5] Hernandez RD, Williamson SH, Bustamante CD (2007) Context dependence, ancestral misidentification, and spurious signatures of natural selection. Mol Biol Evol 24: 1792–1800.

[6] Kent WJ (2002) BLAT—The BLAST-like alignment tool. Genome Res 12: 656–664.

[7] Marth GT, Czabarka E, Murvai J, Sherry ST (2004) The allele frequency spectrum in genome-wide human variation data reveals signals of differential demographic history in three large world populations. Genetics 166: 351–372.

[8] Stephens M, Donnelly P (2003) A comparison of bayesian methods for haplotype reconstruction from population genotype data. Am J Hum Genet 73: 1162–1169.

[9] Kumar S, Filipski A, Swarna V, Walker A, Hedges SB (2005) Placing confidence limits on the molecular age of the human-chimpanzee divergence. Proc Natl Acad Sci U S A 102: 18842–18847.

[10] Hudson RR (2002) Generating samples under a Wright-Fisher neutral model of genetic variation. Bioinformatics 18: 337–338.

[11] International HapMap Consortium, Frazer KA, Ballinger DG, Cox DR, Hinds DA, et al. (2007) A second generation human haplotype map of over 3.1 million SNPs. Nature 449: 851–861.

[12] Waterfall JJ, Casey FP, Gutenkunst RN, Brown KS, Myers CR, et al. (2006) Sloppy-model universality class and the Vandermonde matrix. Phys Rev Lett 97: 150601.

[13] Myers S, Fefferman C, Patterson N (2008) Can one learn history from the allelic spectrum? Theor Popul Biol 73: 342–348.

[14] Price AL, Patterson N, Yu F, Cox DR, Waliszewska A, et al. (2007) A genomewide admixture map for latino populations. Am J Hum Genet 80: 1024–1036.

[15] Nielsen R, Hubisz M, Hellmann I, Torgerson D, Andrés A, et al. Darwinian and demographic forces affecting human protein coding genes. In press.

[16] Pritchard JK, Stephens M, Donnelly P (2000) Inference of population structure using multilocus genotype data. Genetics 155: 945–959.

Table 8: Properties of genes analyzed. Recorded are the location of each gene, the number of noncoding bases sequenced, and the number of SNPs found in that sequence. Note that these are SNPs segregating in any of the EGP populations, of which we've considered subsets. The horizontal lines divide genes that were considered contiguous possibly linked blocks in our simulations with linkage. For each of these 194 blocks, the recombination rate used is reported.

| Gene | Location | Noncoding sequenced | SNPs | Recomb. rate (cM/Mb) |
|---|---|---|---|---|
| tnfrsf4 | chr1:1134785-1141404 | 5785 | 53 | 0.89 |
| eno1 | chr1:8842305-8863311 | 15246 | 83 | 0.26 |
| angptl7 | chr1:11170249-11180532 | 8209 | 56 | 0.05 |
| mad2l2 | chr1:11655241-11665757 | 9026 | 75 | 3.47 |
| ece1 | chr1:21416988-21490465 | 40367 | 234 | 0.99 |
| rpa2 | chr1:28088693-28115249 | 23201 | 142 | 0.21 |
| cdc20 | chr1:43595293-43603425 | 6632 | 21 | 0.04 |
| prdx1 | chr1:45747295-45761481 | 12662 | 89 | 0.08 |
| cyp4b1 | chr1:47035798-47059298 | 15169 | 132 | 0.52 |
| gpx7 | chr1:52839455-52849118 | 8496 | 53 | 0.31 |
| mrpl37 | chr1:54436478-54458642 | 17729 | 111 | 4.22 |
| gstm3 | chr1:110076140-110086554 | 9480 | 52 | 0.45 |
| dclre1b | chr1:114247570-114260035 | 9519 | 38 | 4.74 |
| fmo5 | chr1:145123019-145164842 | 16491 | 117 | 0.30 |
| mcl1 | chr1:148811707-148820540 | 6884 | 26 | 0.09 |
| sprr3 | chr1:151238865-151243575 | 3822 | 54 | 0.01 |
| hspa6 | chr1:159758724-159765190 | 3836 | 74 | 1.09 |
| cd3z | chr1:165665594-165756452 | 35760 | 251 | 5.30 |
| fmo3 | chr1:169324675-169355337 | 19347 | 161 | |
| fmo2 | chr1:169419962-169446946 | 24498 | 201 | 0.56 |
| fmo4 | chr1:169548369-169579838 | 23589 | 90 | 1.52 |
| prdx6 | chr1:171711198-171725810 | 12879 | 73 | 0.17 |
| abl2 | chr1:177341425-177466679 | 30983 | 166 | 0.04 |
| glrx2 | chr1:191330262-191343224 | 10690 | 39 | 0.00 |
| sphar | chr1:227504932-227509818 | 4694 | 21 | 0.00 |
| dclre1c | chr10:14988098-15038104 | 33128 | 283 | 1.29 |
| sirt1 | chr10:69313282-69350134 | 23368 | 135 | 0.06 |
| pten | chr10:89611246-89718010 | 44318 | 171 | 0.04 |
| pdlim1 | chr10:96986027-97042728 | 40888 | 267 | 3.21 |
| mms19l | chr10:99206900-99249416 | 31198 | 133 | 0.28 |
| cyp17a1 | chr10:104578288-104587866 | 6830 | 39 | 0.28 |
| prdx3 | chr10:120915578-120929924 | 12842 | 89 | 1.00 |
| fgfr2 | chr10:123226932-123349844 | 47179 | 321 | 1.92 |
| mmp21 | chr10:127443010-127456384 | 11664 | 68 | 0.47 |
| bnip3 | chr10:133629245-133647430 | 16068 | 88 | 0.21 |
| cyp2e1 | chr10:135188892-135204545 | 10388 | 80 | 1.62 |
| muc2 | chr11:1063774-1096409 | 18417 | 203 | |
| muc5ac | chr11:1130549-1247305 | 43767 | 435 | 8.59 |
| adm | chr11:10281267-10287423 | 5598 | 20 | 0.08 |
| calca | chr11:14945166-14951958 | 5857 | 31 | 0.18 |
| fancf | chr11:22598688-22605597 | 5784 | 36 | 0.26 |
| depc1 | chr11:43857038-43900374 | 21499 | 157 | 0.26 |
| ddb1 | chr11:60821542-60858358 | 24953 | 140 | 0.02 |
| esrra | chr11:63828047-63842665 | 9753 | 44 | |
| prdx5 | chr11:63840191-63847827 | 6991 | 39 | 0.16 |
| fibp | chr11:65406224-65414553 | 7234 | 40 | 0.02 |
| pold4 | chr11:66873631-66879563 | 5608 | 24 | 0.01 |
| fadd | chr11:69724915-69731534 | 5992 | 35 | 0.81 |
| ucp2 | chr11:73362345-73373540 | 8695 | 45 | 0.85 |
| birc2 | chr11:101721227-101756502 | 16890 | 99 | 0.19 |
| mmp8 | chr11:102086541-102102880 | 14746 | 114 | 0.38 |
| mmp12 | chr11:102236716-102252838 | 13144 | 60 | 0.21 |
| casp4 | chr11:104317257-104346525 | 19430 | 124 | |
| casp5 | chr11:104368183-104385539 | 12732 | 96 | 3.07 |
| bace1 | chr11:116659883-116694031 | 28147 | 101 | 0.66 |

| | | | | |
|---|---|---|---|---|
| foxm1 | chr12:2835814-2858359 | 13105 | 84 | 0.44 |
| cd4 | chr12:6767038-6800499 | 20508 | 124 | 3.67 |
| ddit3 | chr12:56195043-56201780 | 5857 | 25 | 0.10 |
| txnrd1 | chr12:103203105-103269990 | 39658 | 208 | 0.09 |
| tuba2 | chr13:18643916-18655936 | 10143 | 134 | 1.53 |
| tgm1 | chr14:23786446-23804157 | 14147 | 84 | 4.81 |
| prkd1 | chr14:29113440-29468639 | 117650 | 709 | 1.01 |
| hspa2 | chr14:64070670-64081266 | 8398 | 50 | 0.26 |
| rad51l1 | chr14:67354260-68014651 | 54253 | 286 | 0.32 |
| mlh3 | chr14:74551067-74589968 | 26770 | 106 | 0.06 |
| ngb | chr14:76799588-76809367 | 8578 | 25 | 0.29 |
| tdp1 | chr14:89489997-89582627 | 54024 | 450 | 0.09 |
| atxn3 | chr14:91597290-91644709 | 33289 | 233 | 0.39 |
| cdc42bpb | chr14:102466485-102594317 | 68463 | 555 | 0.37 |
| ckb | chr14:103053810-103060893 | 4975 | 26 | 0.58 |
| tjp1 | chr15:27777670-27903095 | 64491 | 206 | 0.06 |
| capn3 | chr15:40437058-40493743 | 33273 | 259 | 0.41 |
| lcmt2 | chr15:41405704-41412105 | 4004 | 27 | |
| tp53bp1 | chr15:41484739-41591642 | 42841 | 155 | 0.06 |
| dut | chr15:46409739-46424845 | 14611 | 73 | 0.13 |
| cyp19a1 | chr15:49286972-49420103 | 41602 | 235 | 0.77 |
| aldh1a2 | chr15:56030935-56147219 | 41406 | 297 | 0.21 |
| ppib | chr15:62233067-62244406 | 7645 | 29 | 0.51 |
| cyp1a1 | chr15:72797088-72806750 | 7744 | 41 | |
| csk | chr15:72859819-72884394 | 20901 | 104 | 0.34 |
| blm | chr15:89059760-89160889 | 43775 | 320 | 1.91 |
| abcc1 | chr16:15949029-16144720 | 77618 | 548 | 2.36 |
| itgal | chr16:30390443-30443977 | 32203 | 98 | 1.04 |
| tgfb1i1 | chr16:31390025-31398732 | 6253 | 29 | 0.14 |
| mt3 | chr16:55178288-55185470 | 6383 | 54 | |
| mt2a | chr16:55198077-55202889 | 4315 | 26 | 1.60 |
| mmp15 | chr16:56614812-56639604 | 20075 | 127 | 0.67 |
| ces2 | chr16:65523966-65538512 | 11835 | 34 | 0.10 |
| cdh1 | chr16:67327048-67427588 | 33768 | 192 | 1.03 |
| map2k4 | chr17:11863715-11989045 | 52874 | 244 | 0.78 |
| nos2a | chr17:23105934-23153691 | 40735 | 245 | 0.99 |
| traf4 | chr17:24094767-24102944 | 4920 | 17 | 0.05 |
| slc6a4 | chr17:25547870-25588397 | 32318 | 163 | 1.23 |
| ccl5 | chr17:31220679-31233116 | 8983 | 43 | 0.15 |
| aoc2 | chr17:38248179-38256964 | 5192 | 31 | |
| aoc3 | chr17:38254788-38265391 | 8311 | 53 | 0.91 |
| epx | chr17:53623637-53638737 | 11958 | 66 | |
| mpo | chr17:53700284-53715294 | 12360 | 59 | 1.04 |
| fdxr | chr17:70369763-70382705 | 10034 | 80 | 0.76 |
| flj35220 | chr17:76002438-76028361 | 22577 | 218 | 1.17 |
| tbxa2r | chr19:3543524-3559600 | 8156 | 55 | 2.61 |
| retn | chr19:7638899-7643335 | 3094 | 23 | 12.40 |
| cdc37 | chr19:10360810-10376873 | 9676 | 61 | 0.53 |
| prdx2 | chr19:12767010-12775436 | 6352 | 20 | 0.13 |
| jund | chr19:18249798-18255411 | 4569 | 31 | 0.21 |
| uba52 | chr19:18541857-18551267 | 7682 | 76 | 0.63 |
| cyp2a6 | chr19:46039745-46049329 | 6359 | 24 | 0.85 |
| cyp2b6 | chr19:46188528-46217135 | 12150 | 114 | 0.53 |
| fosb | chr19:50661388-50672275 | 7981 | 48 | 0.62 |
| fgf21 | chr19:53949867-53954694 | 3266 | 26 | 4.08 |
| tpo | chr2:1394275-1527510 | 52005 | 451 | 1.04 |
| odc1 | chr2:10495964-10507871 | 8829 | 77 | 2.89 |
| osr1 | chr2:19412748-19423807 | 10107 | 57 | 3.98 |
| tp53i3 | chr2:24151902-24163166 | 9080 | 37 | 0.02 |
| xdh | chr2:31410740-31492750 | 49855 | 359 | 1.90 |
| srd5a2 | chr2:31601222-31661522 | 25841 | 149 | 0.27 |

| | | | | |
|---|---|---|---|---|
| rev1l | chr2:99381900-99474946 | 47250 | 215 | 0.04 |
| sult1c2 | chr2:108358851-108372202 | 11442 | 57 | 0.22 |
| casp10 | chr2:201753864-201795925 | 36933 | 181 | |
| casp8 | chr2:201804951-201862677 | 25564 | 155 | 0.32 |
| xrcc5 | chr2:216679600-216781263 | 59688 | 377 | 0.33 |
| cdk5r2 | chr2:219530783-219536873 | 4688 | 22 | 0.48 |
| tuba1 | chr2:219821294-219828881 | 5335 | 24 | 0.07 |
| pax3 | chr2:222770789-222873966 | 37987 | 238 | 2.11 |
| ugt1a1 | chr2:234331663-234348269 | 14764 | 102 | 3.88 |
| stk25 | chr2:242082485-242098503 | 11355 | 85 | 1.13 |
| tgm3 | chr20:2222687-2271646 | 27310 | 195 | 14.22 |
| adam33 | chr20:3594643-3612212 | 11441 | 98 | 9.72 |
| gss | chr20:32977941-33008951 | 24298 | 109 | 0.33 |
| tgm2 | chr20:36188289-36228787 | 33377 | 239 | 1.48 |
| plcg1 | chr20:39197582-39239725 | 38122 | 173 | 0.06 |
| mmp9 | chr20:44068952-44080602 | 8530 | 45 | 0.45 |
| ncoa3 | chr20:45562610-45720991 | 67165 | 312 | 0.09 |
| spo11 | chr20:55336692-55354204 | 16068 | 72 | 0.20 |
| chrna4 | chr20:61444524-61465155 | 13979 | 127 | 3.14 |
| app | chr21:26174598-26466748 | 76787 | 422 | 0.96 |
| trpm2 | chr21:44596008-44688231 | 46955 | 256 | 1.77 |
| tbx1 | chr22:18109239-18152828 | 40156 | 324 | 4.01 |
| mapk1 | chr22:20441947-20553900 | 44393 | 223 | 0.06 |
| mmp11 | chr22:22443300-22458501 | 10387 | 83 | |
| smarcb1 | chr22:22457747-22508636 | 29700 | 311 | 0.35 |
| mn1 | chr22:26472295-26529526 | 31530 | 217 | 9.42 |
| mb | chr22:34331272-34345316 | 13084 | 83 | 0.47 |
| rad18 | chr3:8894583-8982157 | 47273 | 353 | 0.35 |
| fancd2 | chr3:10041369-10118048 | 43662 | 291 | 0.03 |
| oxsr1 | chr3:38180035-38273949 | 45330 | 196 | 0.04 |
| cx3cr1 | chr3:39278151-39298493 | 18139 | 123 | 2.52 |
| cxcr6 | chr3:45958001-45966776 | 6418 | 36 | 0.08 |
| poln | chr4:2043284-2202575 | 63537 | 303 | 0.75 |
| ugt2b4 | chr4:70378553-70398209 | 16390 | 128 | 1.27 |
| fgf5 | chr4:81404858-81433179 | 25201 | 225 | 3.66 |
| snca | chr4:90863805-90977228 | 39808 | 283 | 0.17 |
| adh5 | chr4:100209588-100231047 | 19125 | 155 | |
| adh4 | chr4:100263522-100285442 | 17459 | 167 | |
| adh6 | chr4:100342975-100360914 | 16267 | 61 | |
| adh1a | chr4:100415366-100432987 | 14726 | 75 | |
| adh1b | chr4:100446108-100463534 | 14564 | 69 | |
| adh1c | chr4:100474697-100494926 | 12484 | 100 | 0.33 |
| gab1 | chr4:144476938-144612701 | 40223 | 175 | 0.48 |
| anapc10 | chr4:146133771-146240749 | 31273 | 128 | 0.01 |
| neil3 | chr4:178466441-178522793 | 31513 | 236 | 2.59 |
| cyp4v2 | chr4:187347686-187372899 | 19389 | 157 | 3.60 |
| tert | chr5:1304982-1349971 | 27598 | 235 | 3.94 |
| rad1 | chr5:34939140-34956145 | 14622 | 83 | 0.13 |
| sepp1 | chr5:42834018-42849661 | 14107 | 69 | 0.10 |
| xrcc4 | chr5:82407721-82686781 | 76892 | 515 | 0.57 |
| glrx | chr5:95173453-95186148 | 9618 | 72 | 1.99 |
| ube2b | chr5:133732767-133757695 | 22770 | 118 | 0.02 |
| hspa9b | chr5:137917554-137941006 | 17066 | 64 | 0.07 |
| ctnna1 | chr5:138144392-138300374 | 37327 | 178 | 0.04 |
| atox1 | chr5:151100578-151120117 | 16976 | 80 | 0.21 |
| dusp1 | chr5:172125723-172132307 | 4900 | 31 | 1.12 |
| fgfr4 | chr5:176445082-176458717 | 8382 | 45 | 0.52 |
| mapk9 | chr5:179593434-179642220 | 41550 | 270 | 0.44 |
| gpx6 | chr6:28578919-28593498 | 11224 | 69 | |
| gpx5 | chr6:28599802-28611651 | 9891 | 47 | 0.16 |
| msh5 | chr6:31813759-31842569 | 21092 | 108 | |
| hspa1l | chr6:31883771-31891515 | 5083 | 33 | |

| | | | | |
|---|---|---|---|---|
| hspa1a | chr6:31889373-31895694 | 2453 | 17 | |
| hspa1b | chr6:31901538-31907733 | 4013 | 30 | 0.13 |
| fance | chr6:35527645-35544820 | 13668 | 81 | 0.17 |
| gsta3 | chr6:52867429-52884390 | 13987 | 93 | |
| gsta4 | chr6:52950677-52970041 | 14568 | 99 | 2.54 |
| marcks | chr6:114283284-114291631 | 7237 | 24 | 3.17 |
| hsf2 | chr6:122760560-122797817 | 29209 | 108 | 0.04 |
| vnn1 | chr6:133042458-133078042 | 16990 | 141 | |
| vnn3 | chr6:133084723-133099338 | 13790 | 121 | |
| vnn2 | chr6:133104704-133122726 | 14925 | 122 | 3.14 |
| nudt1 | chr7:2248275-2257703 | 8506 | 96 | 0.68 |
| rac1 | chr7:6380405-6412143 | 27091 | 252 | 0.35 |
| rpa3 | chr7:7641155-7726729 | 39301 | 284 | 1.63 |
| polm | chr7:44077383-44090597 | 11122 | 64 | 0.08 |
| igfbp3 | chr7:45916382-45929339 | 11936 | 61 | 5.63 |
| por | chr7:75420622-75454411 | 15593 | 114 | 3.20 |
| hspb1 | chr7:75769508-75772601 | 2475 | 20 | 1.28 |
| abcb4 | chr7:86867353-86949645 | 69500 | 410 | |
| abcb1 | chr7:86970771-87182449 | 88991 | 468 | 0.41 |
| cyp3a5 | chr7:99083564-99115770 | 16185 | 76 | |
| cyp3a4 | chr7:99191632-99221666 | 20737 | 67 | 0.50 |
| abp1 | chr7:150178590-150191285 | 8699 | 55 | 2.11 |
| slc4a2 | chr7:150385719-150406496 | 15421 | 103 | 1.09 |
| msr1 | chr8:16008774-16094804 | 24853 | 268 | 3.76 |
| scara3 | chr8:27545520-27588149 | 37814 | 303 | 1.02 |
| ube2v2 | chr8:49082972-49138936 | 15669 | 41 | 0.05 |
| terf1 | chr8:74081659-74123686 | 29263 | 205 | 0.10 |
| mmp16 | chr8:89120172-89410308 | 70209 | 382 | 0.91 |
| rrm2b | chr8:103284760-103322295 | 30205 | 164 | 0.45 |
| oxr1 | chr8:107739110-107833889 | 37475 | 141 | 0.05 |
| cyc1 | chr8:145220372-145226365 | 4786 | 26 | 0.07 |
| recql4 | chr8:145705653-145715945 | 6665 | 61 | 0.41 |
| ifna1 | chr9:21428453-21432913 | 3554 | 36 | 0.36 |
| dapk1 | chr9:89300614-89513612 | 97580 | 718 | 3.56 |
| fbp1 | chr9:96403244-96443887 | 30956 | 258 | 0.37 |
| ptch | chr9:97244275-97311000 | 33249 | 175 | 0.87 |
| pole3 | chr9:115207883-115214172 | 5845 | 36 | 0.26 |
| hspa5 | chr9:127035208-127045070 | 7560 | 39 | 0.23 |
| ciz1 | chr9:129966204-130008434 | 21746 | 139 | 0.64 |
| abl1 | chr9:132577087-132753794 | 52704 | 371 | 0.87 |
| rxra | chr9:136431296-136474254 | 32537 | 351 | 1.99 |
